# Supplementary material for: Temperature-dependent spin-transport and current-induced torques in superconductor/ferromagnet heterostructures
Source: arXiv:2007.15569 ancillary file (2020-07-30)
Supplement: Supplementary file 1 [file Supplements.pdf]

# Temperature-dependent spin-transport and current-induced torques in superconductor/ferromagnet heterostructures

M. Müller,[1,2,*] L. Liensberger,[1,2] L. Flacke,[1,2] H. Huebl,[1,2,3] A. Kamra,[4] W. Belzig,[5] R. Gross,[1,2,3] M. Weiler,[1,2] and M. Althammer[1,2,†]

[1] *Walther-Meißner-Institut, Bayerische Akademie der Wissenschaften, 85748 Garching, Germany*
[2] *Physik-Department, Technische Universität München, 85748 Garching, Germany*
[3] *Munich Center for Quantum Science and Technology (MCQST), Schellingstr. 4, 80799 München, Germany*
[4] *Center for Quantum Spintronics, Department of Physics, Norwegian University of Science and Technology, NO-7491 Trondheim, Norway*
[5] *Fachbereich Physik, Universität Konstanz, 78457 Konstanz, Germany*
(Dated: July 30, 2020)

## 1. SAMPLE FABRICATION AND GROWTH PARAMETERS

The growth of functional high quality superconductor/ferromagnet heterostructures imposes high demands on the used ultra high vacuum machine as an in situ deposition of both layers is favourable for clean SC/FM-interfaces. We utilize our Superbowl ultra-high-vacuum machine manufactured by Bestec GmbH to grow both ferromagnetic and non-magnetic/superconducting materials in two separate deposition chambers as illustrated in Fig. S1. We use the SP2 chamber (highlighted in blue) to grow superconducting NbN and then transfer the sample through the evacuated loadlock into the SP4 chamber (highlighted in red) to grow a low-damping FM. The base pressure in both deposition chambers after bakeout is $< 7 \cdot 10^{-10}$ mbar.

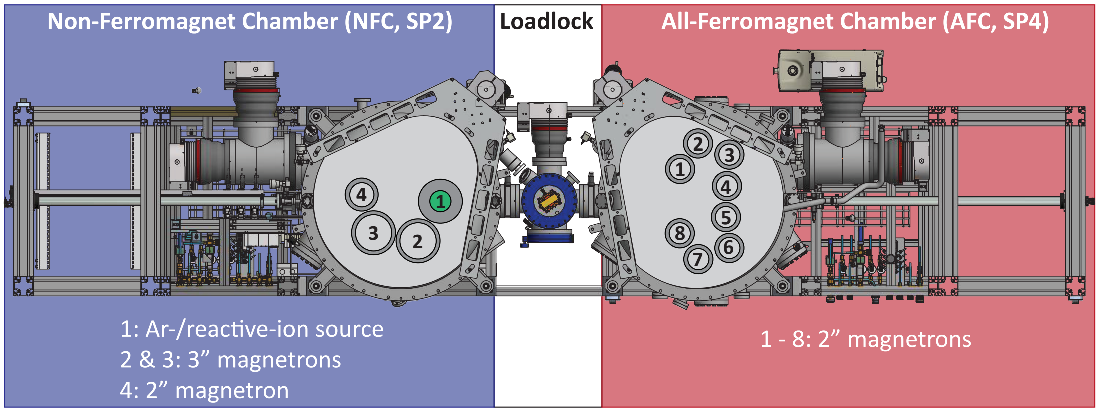


Figure S1. Sketch of the Superbowl sputtering machine.

Our SC/FM-heterostructures were grown on cleaned Si (001) substrate with a 1 µm thick thermally grown $SiO_2$-capping layer on top. We selected NbN as our superconducting layer for its resilience to magnetic fields and high superconducting transition temperature of up to $T_C$ =16.8 K [1–3]. These properties make NbN an ideal candidate for bbFMR at cryogenic temperatures as it offers both a large margin in $T$ between the boiling point of liquid helium and $T_C$ and also in applied external field $\mu_0 H_{ext}$, which directly translates to the bandwidth of applicable driving frequencies $f$ in bbFMR. We grew NbN both on the bare substrate and several heavy metals like Pt to investigate its spin pumping properties.
After the deposition of NbN in the SP2 chamber, the substrate is transferred to the SP4 chamber for the growth of a low-damping ferromagnetic material. Here, we chose the alloy $Ni_{80}Fe_{20}$ (Permalloy, Py). Lastly, we deposited a thin capping layer of Ta on our FM to protect it from oxidization.
The respective sputtering parameters of the individual materials are listed in Tab. S1

| Target material | $P$ [W] | $r$ [Å/s] | $T$ [°C] | $N_2$/Ar-ratio |
|---|---|---|---|---|
| Al | 40 | 1.4 | RT | - |
| $Co_{25}Fe_{75}$ | 25 | 1.0 | RT | - |
| Cu | 30 | 1.3 | RT | - |
| NbN | 120 | 4.0 | 400 | 1.9/18.1 |
| Py | 80 | 2.1 | RT | - |
| Pt | 30 | 4.2 | RT | - |
| Ta | 30 | 0.5 | RT | - |

Table S1. Sputtering parameters of the materials grown in the Superbowl. All materials were grown at an Ar-pressure $p = 5 \times 10^{-3}$ mbar

For our SC/FM-heterostructures the goal was to detect and quantify the spin current $\mathbf{J}_\mathrm{s}$ injected from our FM via spin pumping into the Pt layer by investigating the iSHE and comparing it for samples with and without spin sink layer. To this end, we adjusted the layer thickness of NbN $d_\mathrm{SC}$ to maintain a reasonable $T_\mathrm{c}$ and to increase the $\mathbf{J}_\mathrm{s}$ entering the Platinum. We hence reduced $d_\mathrm{SC}$ to 16 nm. Additionally, we prepared samples by inserting a Pt buffer layer between NbN and Py to investigate the nature of the observed field-like iSOT. We utilized Pt buffer layers of varying thickness, which besides lifting the FM/SC proximity also absorb spin currents injected from the Py layer. Hence, the insertion of a thick Pt buffer layer should ensure an unperturbed superconducting NbN only affected by the oscillatory microwave field. Finally, we used Py as our FM for its resilient growth properties, which enables us to grow our FM on top of several different materials with unaffected magnetization dynamics parameters. This ensures comparability between our samples. Here we chose a layer thickness of $d_\mathrm{SC}$ to 6 nm to ensure a reasonable signal-to-noise ratio (SNR) for our FMR.

## 2. DETERMINATION OF THE SUPERCONDUCTING TRANSITION TEMPERATURE

To determine $T_\mathrm{c}$, we recorded $|\mathrm{S}_{21}|$ at a fixed frequency of 30 GHz as a function of sample temperature. The results are shown in Fig. S2.

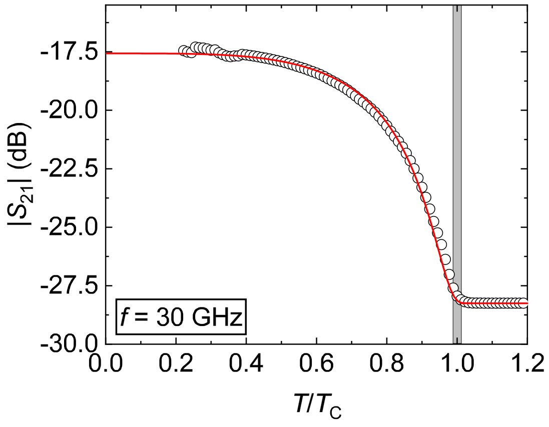


Figure S2. The recorded $|S_{21}|$ at a fixed microwave frequency $f$ =30 GHz is shown as a function of normalized temperature for sample B. It steeply increases once the NbN-layer becomes superconducting and is fitted using Eq. (S4) to extract the London penetration depth $\lambda_\mathrm{L}$ =(1.12 ± 0.06) µm.

As the observed changes in $|\mathrm{S}_{21}|$ manifest abruptly and no further alterations occur for $T > T_\mathrm{c}$, it is reasonable to presume that the changes in $|\mathrm{S}_{21}|$ are indeed caused by the onset of superconductivity. For a quantitative description of the observed behaviour we used the results of Schmidt *et. al.* in [4]. They derived an expression for $|\mathrm{S}_{21}|$ normalized by the transmission parameter of an unloaded CPW $|\mathrm{S}^0_{21}|$.

$$\left|\frac{S_{21}}{S^0_{21}}\right| \propto \exp\left(-\frac{|\gamma_0 Z_\mathrm{eff}|l}{2Z_0}\right). \tag{S1}$$

Here, $l$ represents the sample's length on the CPW, $Z_{\rm eff}$ and $Z_0$ stand for the thin film surface impedance and unloaded CPW-impedance, respectively. Additionally, $\gamma_0 = {}^{\omega}/_{v_{\rm ph}}$ is the complex propagation factor, where $f = {}^{\omega}/_{2\pi}$ and $v_{\rm ph}$ is the phase velocity of microwaves in the CPW. For $Z_{\rm eff}$, we use [5, 6]

$$Z_{\rm eff}(\omega) = \frac{1}{2}\mu_0^2\omega^2\lambda_{\rm eff}^3\sigma_0\frac{n_{\rm n}}{n} - i\cdot\mu_0\omega\lambda_{\rm eff} \tag{S2}$$

Here, $\sigma_0$ is the conductance of the SC layer in the normal state, $n_{\rm n}/n$ is the fraction of the normal-conducting phase below $T_{\rm c}$ and $\lambda_{\rm eff} = \lambda_{\rm L}^2/d_{\rm SC}$ is the thin film London penetration depth [7]. We simplify Eq. (S2) by only considering its imaginary part, which is the dominant contribution for temperatures not too close to the transition temperature. The $T$-dependence of $|S_{21}|$ is then just governed by that of the London penetration depth $\lambda_{\rm L}$, most commonly described by the Casimir-Görter-model [8]:

$$\lambda_{\rm L}(T) = \frac{\lambda_{\rm L}(0)}{\sqrt{1-(T/T_{\rm c})^4}} \tag{S3}$$

By inserting Eq. (S2) into (S1) and taking its temperature dependence into account, we obtain the final result

$$|S_{21}| = |S_{21}^{\rm NC}| + |\Delta S_{21}|\exp\left(-\frac{|\gamma_0| l\mu_0\omega\lambda_{\rm L}^2(0)}{2Z_0 d_{\rm SC}(1-(T/T_{\rm c})^4)}\right) \tag{S4}$$

for our fitting function with $|S_{21}^{\rm NC}|$ representing the complex transmission magnitude in the normalconducting range and $|\Delta S_{21}|$ being its change below $T_{\rm c}$. The resulting fit curve is shown in Fig. S2. When applying the values $d_{\rm SC}$ = 16 nm, $l$ = 6 mm, $v_{\rm ph} = 1.8\cdot 10^8$ m/s (used by Schmidt et. al. in Ref. [4]) and $Z_0$ =50 Ω, the extracted London penetration depth is $\lambda_{\rm L}$ =(1.12 ± 0.06) µm, which is considerably larger than literature values for NbN, ranging from 200 nm to 400 nm [2, 3]. However, a correction factor according to [9] must be applied of the form

$$\lambda_{\rm L}(0) = \lambda_{\rm L}^{\infty}(0)\left(1+\frac{\xi^{\infty}(0)}{l_0}\right)^{1/2}, \tag{S5}$$

where $\xi^{\infty}$ and $l_0$ are the bulk SC coherence length and mean free path respectively. Using $l_0$ =3.96 Å[10], $\xi^{\infty}$ = 5 nm [11] and $\lambda_{\rm L}^{\infty}(0)$ = 300 nm, we obtain $\lambda_{\rm L}(0) \approx 1$ µm, which agrees well with our experimental results. It should be noted that an unusually large $\lambda_{\rm L}$ has been observed for SC/FM-bilayers in [12], where it was attributed to the depletion of the superconducting fluid density $n_{\rm s}$ at the FM interface. However, in our samples the large $\lambda_{\rm L}$ may as well be explained by finite size effects and a reduction in the superconducting coherence length $\xi_0$ due to changes in the normalconducting mean free path of the superconducting layer. The respective $T_{\rm c}$ and $\lambda_{\rm L}$ of all samples, which were included in the main text, are listed in Tab. S2.

| Sample | **A** | **B** | **C** | **D** |
|---|---|---|---|---|
| $T_{\rm c}$ [K] | 11.5 | 9.0 | 10.0 | 10.2 |
| $\lambda_{\rm L}$ [$\mu$m] | 0.84 | 1.12 | 0.71 | 0.96 |

Table S2. Superconducting transition temperature $T_{\rm c}$ and estimated London penetration depth $\lambda_{\rm L}$ of samples discussed in the main text.

## 3. FERROMAGNETIC RESONANCE

We start with the LLG equation [13]

$$\frac{\mathrm{d}\mathbf{M}}{\mathrm{dt}} = -\gamma \mathbf{M} \times \mu_0 \mathbf{H}_{\mathrm{eff}} + \frac{\alpha}{\mathrm{M_s}} \mathbf{M} \times \frac{\mathrm{d}\mathbf{M}}{\mathrm{dt}}, \tag{S6}$$

where $\alpha$ is the Gilbert damping parameter and $\gamma = g\mu_{\mathrm{B}}/\hbar$ is the gyromagnetic ratio. $\mathbf{H}_{\mathrm{eff}} = \mathbf{H}_{\mathrm{ext}} + \mathbf{H}_{\mathrm{de}} + \mathbf{H}_{\mathrm{ani}}$ is the effective field with anisotropy field $\mathbf{H}_{\mathrm{ani}}$ and demagnetizing field $\mathbf{H}_{\mathrm{de}}$. $\mathbf{M} \times \frac{\mathrm{d}\mathbf{M}}{\mathrm{dt}}$ is directed towards the rotation center, effectively reducing the precession amplitude as a function of time. The resulting trajectory for $\mathbf{M}$ is a spiral motion around $\mathbf{H}_{\mathrm{eff}}$.

We describe the response of a finite sample with magnetization $\mathbf{M}$ exposed to a constant external magnetic field applied along the x-axis $\mathbf{H} = H_{\mathrm{ext}}\hat{\mathbf{e}}_{\mathrm{x}}$ and driven by an oscillatory field $\mathbf{h}_{\mathrm{rf}}$ in the yz–plane, triggering a dynamic response $\mathbf{m}(t)$ in the ferromagnet. Under these circumstances, we can split the magnetic field $\mathbf{H}_{\mathrm{eff}}$ and magnetization $\mathbf{M}$ into a time-independent and a time-dependent part:

$$\begin{aligned} \mathbf{H}_{\mathrm{eff}} &= \mathbf{H}_{\mathrm{ext}} + \mathbf{H}_{\mathrm{ani}} - \mathbf{H}_{\mathrm{de}} + \mathbf{h}_{\mathrm{rf}}(t) = (H_{\mathrm{ext}} + H_{\mathrm{ani}} - N_{\mathrm{x}} M_0)\hat{\mathbf{e}}_{\mathrm{x}} + \mathbf{h}_{\mathrm{rf}}(t) \\ \mathbf{M} &= \mathbf{M}_0 + \mathbf{m}(t) = M_0 \hat{\mathbf{e}}_{\mathrm{x}} + \mathbf{m}(t) \end{aligned} \tag{S7}$$

A linear approach of the form

$$\begin{aligned} \mathbf{h}_{\mathrm{rf}}(t) &= (h_{\mathrm{rf,y}}\hat{\mathbf{e}}_{\mathrm{y}} + h_{\mathrm{rf,z}}\hat{\mathbf{e}}_{\mathrm{z}}) \cdot e^{i\omega t} \\ \mathbf{m}(t) &= (m_{\mathrm{y}}\hat{\mathbf{e}}_{\mathrm{y}} + m_{\mathrm{z}}\hat{\mathbf{e}}_{\mathrm{z}}) \cdot e^{i\omega t}, \end{aligned} \tag{S8}$$

is used for the time-dependent contributions under the premise, that $m_{\mathrm{y/z}} \ll M_0$.

This Ansatz is plugged into the LLG (S6), where we assume, that the static part of the magnetization $\mathbf{M}_0$ is parallel to the external field and hence $\mathbf{M}_0 \times \mathbf{H}_{\mathrm{ext}} = 0$. The resulting expression

$$\begin{pmatrix} h_{\mathrm{rf,y}} \\ h_{\mathrm{rf,z}} \end{pmatrix} = \hat{\chi}_{\mathrm{P}}^{-1} \begin{pmatrix} m_{\mathrm{y}} \\ m_{\mathrm{z}} \end{pmatrix} \tag{S9}$$

provides the Polder susceptibility [14].

$$\begin{aligned} \hat{\chi}_{\mathrm{P}} &= \frac{\mu_0 M_{\mathrm{s}}}{\mathrm{Det}(\hat{A})}\hat{A}\ , \text{ with} \\ \hat{A} &= \begin{pmatrix} A_{11} & \frac{i\omega}{\gamma\mu_0} \\ -\frac{i\omega}{\gamma\mu_0} & A_{22} \end{pmatrix} \\ A_{11} &= H_{\mathrm{ext}} + H_{\mathrm{ani}} + M_{\mathrm{s}} \cdot (N_{\mathrm{y}} - N_{\mathrm{x}}) + \frac{i\omega\alpha}{\gamma\mu_0} \\ A_{22} &= H_{\mathrm{ext}} + H_{\mathrm{ani}} + M_{\mathrm{s}} \cdot (N_{\mathrm{z}} - N_{\mathrm{x}}) + \frac{i\omega\alpha}{\gamma\mu_0} \end{aligned} \tag{S10}$$

In ip-geometry, the Polder-susceptibility $\hat{\chi}_{\mathrm{P}}$ (S10) takes the following form [$N_{\mathrm{z}}$ =1, $N_{\mathrm{x}}$ =0, $N_{\mathrm{y}}$ =0]:

$$\begin{aligned} \hat{\chi}_{\mathrm{P}} &= \begin{pmatrix} \chi_{\mathrm{yy}} & \chi_{\mathrm{yz}} \\ \chi_{\mathrm{zy}} & \chi_{\mathrm{zz}} \end{pmatrix} = \frac{\mu_0 M_{\mathrm{s}}}{D} \begin{pmatrix} H_{\mathrm{ext}} + H_{\mathrm{ani}} + i\frac{\Delta H}{2} & +\frac{i\omega}{\mu_0\gamma} \\ -\frac{i\omega}{\mu_0\gamma} & H_{\mathrm{ext}} + M_{\mathrm{s}} + H_{\mathrm{ani}} + i\frac{\Delta H}{2} \end{pmatrix} \\ D &= \left(H_{\mathrm{ext}} + M_{\mathrm{s}} + H_{\mathrm{ani}} + i\frac{\Delta H}{2}\right)\left(H_{\mathrm{ext}} + H_{\mathrm{ani}} + i\frac{\Delta H}{2}\right) - \left(\frac{\omega}{\mu_0\gamma}\right)^2 \end{aligned} \tag{S11}$$

Here we use the abbreviation $\Delta H = \frac{2\omega\alpha}{\gamma\mu_0}$. In this geometry, we detect the combined ferromagnetic response of the two diagonal susceptibility components $\chi_{\mathrm{yy}}$ and $\chi_{\mathrm{zz}}$. Hence, we have to include the ellipticity $\epsilon$ of the precession cone using

$$\hat{\chi}_{\mathrm{ip}} = \hat{\chi}_{\mathrm{zy,ip}} \begin{pmatrix} i\epsilon & -1 \\ 1 & i/\epsilon \end{pmatrix} \tag{S12}$$

with

$$\epsilon = \sqrt{1 + \frac{\mu_0 M_\mathrm{s}}{\mu_0 H_\mathrm{ext}}}. \tag{S13}$$

Here, we neglect any additional anisotropy contributions and only account for the shape anisotropy of the FM in the thin film limit.
We can determine the resonance frequency $f_\mathrm{res}$ as a function of $\mathbf{H}_\mathrm{ext}$ by solving $\mathrm{Det}(\hat{\chi}_\mathrm{ip}) \overset{!}{=} 0$ and taking the real part. In the in-plane-geometry [ip], the external field $\mathbf{H}_\mathrm{ext}$ is applied in the sample plane e.g. along the x-axis with $N_\mathrm{z} = 1$ and $N_\mathrm{x} = N_\mathrm{y} = 0$. The in-plane Kittel equation can be expressed as

$$f = \frac{\gamma\mu_0}{2\pi}\sqrt{(H_\mathrm{ext} + H_\mathrm{ani})(H_\mathrm{ext} + H_\mathrm{ani} + M_\mathrm{eff})}, \tag{S14}$$

where we utilize the effective magnetization $M_\mathrm{eff} = M_\mathrm{s} - H_\mathrm{k}$ of our thin film samples instead of the bulk saturation magnetization $M_\mathrm{s}$ to account for out-of-plane anisotropy $\mathrm{H_k}$ often found in polycrystalline thin films. In our experiments, we sweep the applied field $H_\mathrm{ext}$ at constant frequency $f$ through the resonant field $H_\mathrm{res}$. The required $H_\mathrm{res}$ for a given $f$ is derived by solving Eq. (S14) by $H_\mathrm{ext}$

$$\mu_0 H_\mathrm{res} = -\mu_0 H_\mathrm{ani} - \frac{\mu_0 M_\mathrm{eff}}{2} + \sqrt{\left(\frac{\mu_0 M_\mathrm{eff}}{2}\right)^2 + \left(\frac{2\pi f}{\gamma}\right)^2}, \tag{S15}$$

Apart from the resonance field $H_\mathrm{res}$ at a given frequency $f$, the Polder susceptibility also provides insight into the damping of the ferromagnetic precession in its imaginary part. By using Eq. (S10) and solving $\mathrm{Det}(\hat{\chi}_\mathrm{ip}) \overset{!}{=} 0$ for its imaginary part, we obtain a formula describing the fanning out of the Lorentzian resonance peak as a function of driving frequency

$$\Delta H_\mathrm{FWHM} = 2\frac{2\pi f\alpha}{\gamma\mu_0}, \tag{S16}$$

where $\Delta H_\mathrm{FWHM}$ is its full width at half maximum, whereas $\alpha$ represents the phenomenological damping parameter that comprises all possible damping processes linear in $f$. Following the usual approach, we consider inhomogeneous broadening by using

$$\mu_0 \Delta H = \mu_0 H_\mathrm{inh} + 2 \cdot \frac{2\pi f\alpha}{\gamma}. \tag{S17}$$

for fitting of our experimental data. To extract $\alpha$, we first fit $\mu_0 H_\mathrm{res}$ to Eq. (S15) and then use the extracted $\gamma$ when fitting $\Delta H$ to Eq. (S17).

## 4. THE BROADBAND FERROMAGNETIC RESONANCE TECHNIQUE

In our experiments, the sample is placed face-down on the CPW and the ferromagnetic resonance is excited by a microwave signal generated at port 1 of the VNA and coupled into the CPW via microwave cables attached to endlaunches. In resonance, the sample can absorb energy and we detect a change in the transmitted signal arriving at port 2 due to Faradays law of induction ($V_\mathrm{ind} = -\partial\Phi/\partial t$). We employ transmission measurements, where a microwave signal is generated at port 1 and detected at port 2. To this end, we measure the complex transmission parameter $S_{21}$ defined as

$$S_{21} = \frac{V_2}{V_1} = \frac{|V_2|}{|V_1|} e^{i(\phi_2 - \phi_1)}, \tag{S18}$$

where $V_\mathrm{j}$ are the measured complex voltages with magnitude $|V_\mathrm{j}|$ and phase $\phi_\mathrm{j}$ of the respective port j. It consists of the background $S_{21}^0$ caused by the setup and a change of transmission $\Delta S_{21}$ caused by the sample. The latter is given by

$$\Delta S_{21} = \frac{S_{21} - S_{21}^0}{S_{21}^0}, \tag{S19}$$

when presuming a fully impedance-matched rf circuit and neglecting the back-reflected wave $S_{11}$. To account for the background $S_{21}^0$, we fit a linear function $S_{21}^0 = C_0 + C_1 H_\mathrm{ext}$ with the complex offset $C_0$ and slope $C_1$ following the approach by Nembach *et. al.* in [15]. Upon dividing the susceptibility by $\mu_0 M_\mathrm{s}$, to stay consistent with the formalism in [16], we obtain the final result for our fitting function

$$S_{21}(H_\mathrm{ext})|_\omega = C_0 + C_1 \cdot H_\mathrm{ext} - iAe^{i\phi} \cdot \frac{\chi_\mathrm{yy}(H_\mathrm{ext}) + \zeta\chi_\mathrm{zz}(H_\mathrm{ext})}{\mu_0 M_\mathrm{s}}. \tag{S20}$$

Here, $A$ is the resonance amplitude and $\phi$ is the resonance phase. In the FM, screening currents can particularly attenuate the z-component of the driving field $\mathbf{h}_\mathrm{rf,z}$ [17–19], hence we account for the varying driving field strengths between y- and z-component with the constant factor $\zeta$. The chosen magnitude and impact of varying $\zeta$ on our results are discussed in Section 13. Finally, we we solve Eq. (S20) for $\Delta S_{21}$ as defined in Eq. (S19)

$$\Delta S_{21} = \frac{S_{21} - S_{21}^0}{S_{21}^0} = -i\frac{Ae^{i\Phi}}{C_0 + C_1 H_\mathrm{ext}}\frac{[\chi_\mathrm{yy}(\omega, H_\mathrm{ext}) + \zeta\chi_\mathrm{zz}(\omega, H_\mathrm{ext})]}{\mu_0 M_\mathrm{s}}. \tag{S21}$$

## 5. INDUCTIVE DETECTION OF CURRENT-INDUCED TORQUES

The magnetic driving field $\mathbf{h}_\mathrm{rf}$ in the y-z-plane is generated by an ac charge current through the center conductor, which is a metallic thin film strip with a width $\mathrm{w_{cc}} \simeq 60$ µm. The induced rf-field can be approximated by the Karlqvist equations [16].

$$\begin{aligned} h_\mathrm{y}(\mathrm{y,z}) &= \frac{1}{\pi}\left[\arctan\left(\frac{\mathrm{y} + \frac{w_\mathrm{cc}}{2}}{\mathrm{z}}\right) - \arctan\left(\frac{\mathrm{y} - \frac{w_\mathrm{cc}}{2}}{\mathrm{z}}\right)\right] \\ h_\mathrm{z}(\mathrm{y,z}) &= \frac{1}{2\pi} h_0 \ln\left(\frac{(\mathrm{y} + \frac{w_\mathrm{cc}}{2})^2 + \mathrm{z}^2}{(\mathrm{y} - \frac{w_\mathrm{cc}}{2})^2 + \mathrm{z}^2}\right) \end{aligned} \tag{S22}$$

Here $h_0 = I_\mathrm{CPW}/(2w_\mathrm{cc})$ is the field amplitude at the center for y=z=0 with $= I_\mathrm{CPW}$ as the current flowing in the CPW. This oscillating magnetic field drives the precession of the sample's magnetization and in resonance it induces opposing currents in the CPW according to Faraday's law and hence microwave power is absorbed. By assuming that the sample's inductive coupling adds a complex inductance $L$ in series with the impedance $Z_0$ =50 Ω of the unloaded CPW in a voltage divider model, we can relate the background-corrected change in transmission $\Delta S_{21}$ to $L$ [16]:

$$\Delta S_{21} = -i\frac{\pi f L}{Z_0} \tag{S23}$$

The factor 1/2 is required, as the the complex voltage $V_2$ is measured between CPW and port 2 and not between the two ports.
The sample's inductance $L$ is given by [16]

$$L = L_0 + L_\mathrm{j}, \tag{S24}$$

where $L_0$ is a measure of the coupling strength between the FM and the CPW and $L_\mathrm{j}$ accounts for the flux generated by ac-currents in the adjacent NM/SC-layer. The inductive coupling between FM and CPW, $L_0$ can be calculated with [16]

$$L_0 = \frac{\mu_0 l d_\mathrm{FM}}{4w_\mathrm{cc}}[\chi_\mathrm{yy}(f, H_\mathrm{ext}) + \zeta\chi_\mathrm{zz}(f, H_\mathrm{ext})]\eta^2(\delta_\mathrm{s}, w_\mathrm{cc}), \tag{S25}$$

where $l$ is the sample length on the CPW. We adapt the expression for $L_0$ in [16], by accounting for both susceptibility components $\chi_\mathrm{yy}$ and $\chi_\mathrm{zz}$ in the in-plane geometry. The function $\eta(\delta_\mathrm{s}, w_\mathrm{cc})$ accounts for a finite spacing $\delta_\mathrm{s}$ between sample and coplanar waveguide. It can take values from 1, when they are in direct contact, to zero at infinite distance and is obtained by using Eq. (13) and Eq. (14) in [16].

$$\eta(\delta_\mathrm{s}, w_\mathrm{cc}) = \frac{2}{\pi}\arctan\left(\frac{w_\mathrm{cc}}{2\delta_\mathrm{s}}\right). \tag{S26}$$

In multilayer ferromagnet/non-magnet (FM/NM)-heterostructures, the dipolar contribution $L_0$ of the FM is not the singular source of inductive coupling $L$ between sample and CPW. An additional contribution $L_\mathrm{j} \neq 0$ is generated whenever electrical ac currents flow in the adjacent NM layers as a result of the magnetization precession within the FM. For the inductive method to analyze iSOT, we insert Eq. (S21) into Eq. (S23), which relates $\Delta S_{21}$ to the inductive coupling strength $L$ between sample and CPW and obtain

$$\tilde{L} = \frac{1}{\mu_0 M_\mathrm{s}} \frac{A e^{i\Phi}}{C_0 + C_1 H_\mathrm{ext}} \frac{Z_0}{\pi f}, \tag{S27}$$

where we introduced the normalized inductance $\tilde{L} = L/[\chi_\mathrm{yy}(f, H_\mathrm{ext}) + \zeta \chi_\mathrm{zz}(f, H_\mathrm{ext})]$.

$\tilde{L} = \tilde{L}_0 + \tilde{L}_\mathrm{j}$ in real and imaginary part can be described with

$$\begin{aligned} \mathrm{Re}(\tilde{L}) &= \tilde{L}_0 + \mathrm{Re}(\tilde{L}_\mathrm{j}) = \tilde{L}_0 + \mathrm{Re}(\Delta\tilde{L}_\mathrm{j}) \cdot f \cdot \epsilon_\mathrm{r}(f) \\ \mathrm{Im}(\tilde{L}) &= \mathrm{Im}(\tilde{L}_\mathrm{j}) = \mathrm{Im}(\Delta\tilde{L}_\mathrm{j}) \cdot f \cdot \epsilon_\mathrm{i}(f). \end{aligned} \tag{S28}$$

We distinguish between the frequency-independent normalized inductive coupling strength offset $\tilde{L}_0$ between ferromagnetic layer and center conductor. It can be obtained by dividing the result for $L_0$ in Eq. (S25) by the susceptibility components $[\chi_\mathrm{yy}(\omega, H_0) + \zeta\chi_\mathrm{zz}(\omega, H_0)]$. The second term is the linear change in $\tilde{L}$ with frequency $\Delta\tilde{L}_\mathrm{j}$, which stems from currents flowing in the normal metal that are induced by the oscillating part of the magnetization $\partial\mathbf{m}/\partial t$ and are hence linear in frequency. This result is equal to that in [16] apart for the functions $\epsilon_\mathrm{r}(f)$ and $\epsilon_\mathrm{i}(f)$, which account in real and imaginary part for the elliptical magnetization precession cone of $\mathbf{M}$ in in-plane geometry.
By extracting $\Delta\tilde{L}_\mathrm{j}$ we can extract the current-induced torque conductivity $\sigma^\mathrm{SOT}$, which is a complex quantity that comprises both field- and damping like current-induced torques. In analogy to Ohm's law $\mathbf{J} = \sigma\mathbf{E}$, it relates $\partial\mathbf{m}/\partial t$ to the charge current in the normal metal $\mathbf{J}_\mathrm{j}$[16]

$$\sigma^\mathrm{SOT} = \sigma_\mathrm{f} + i\sigma_\mathrm{d}. \tag{S29}$$

Here 'f' and 'd' denote the field- and damping-like current-induced torques respectively. The former corresponds to both Faraday 'F' and inverse Rashba-Edelstein effect $\sigma_\mathrm{f} = \sigma_\mathrm{f}^\mathrm{iREE}$-$\sigma_\mathrm{f}^\mathrm{F}$, while the latter $\sigma_\mathrm{d}$ primarily quantifies the inverse spin Hall effect. In our samples $\sigma_\mathrm{d}$ is primarily created by the conversion of spin currents originating from the spin pumping into heavy metals like e.g. Pt with large SOI.
The relation between $L_\mathrm{j}$ and $\sigma_\mathrm{SOT}$ is given by [16].

$$L_\mathrm{j} = -L_{12} \frac{\hbar w_\mathrm{cc}}{2eI_\mathrm{CPW}} \hat{\mathbf{e}}_\mathrm{x} \cdot \left[ \hat{\mathbf{e}}_\mathrm{z} \times \frac{\partial\mathbf{m}}{\partial t} \sigma_\mathrm{f} - \hat{\mathbf{e}}_\mathrm{z} \times \left( \mathbf{m} \times \frac{\partial\mathbf{m}}{\partial t} \right) \sigma_\mathrm{d} \right]. \tag{S30}$$

Here, $L_{12}$ is the mutual inductance between sample and CPW. We follow the approach by Rosa in [20] and model the NM/SC and center conductor of the CPW as two current-carrying sheets of width $w_\mathrm{cc}$, length $l$ and separation $\delta_\mathrm{s}$, which provides a mutual inductance $L_{12}$ of

$$L_{12} = \frac{\mu_0}{4\pi} 2l \left[ \ln\left( \frac{2l}{R} - 1 \right) \right], \tag{S31}$$

where $R$ is given by

$$R = \sqrt{w_\mathrm{cc}^2 + \delta_\mathrm{s}^2} \left( \frac{\delta_\mathrm{s}}{\sqrt{w_\mathrm{cc}^2 + \delta_\mathrm{s}^2}} \right)^{\left(\frac{\delta_\mathrm{s}}{w_\mathrm{cc}}\right)^2} \exp\left[ \frac{\delta_\mathrm{s}}{w_\mathrm{cc}} \arctan\left( \frac{\delta_\mathrm{s}}{w_\mathrm{cc}} \right) - \frac{3}{2} \right]. \tag{S32}$$

$L_\mathrm{j}$ is normalized by the contributing susceptibility components to provide the normalized coupling $\tilde{L}_\mathrm{j}$ between NM or SC layer and CPW

$$\tilde{L}_\mathrm{j} = \frac{L_\mathrm{j}}{\chi}. \tag{S33}$$

Note that for didactic purposes, we chose to use the quantity $\tilde{L}_\mathrm{j}$, which we defined as $\tilde{L}_\mathrm{j} = i\tilde{L}_\mathrm{NM}$.
For the **ip**-case with CC$\|\mathbf{H}_\mathrm{ext} \parallel \hat{\mathbf{e}}_\mathrm{x}$, we derive:

$$\mathbf{m} = \left(1,\ \tfrac{1}{M_\mathrm{s}}(\hat{\chi} \cdot \mathbf{h}_\mathrm{rf})_\mathrm{y},\ \tfrac{1}{M_\mathrm{s}}(\hat{\chi} \cdot \mathbf{h}_\mathrm{rf})_\mathrm{z}\right) \tag{S34}$$

$$\frac{\partial \mathbf{m}}{\partial t} = \left(0,\ \tfrac{i\omega}{M_\mathrm{s}}(\hat{\chi}\cdot\mathbf{h}_\mathrm{rf})_\mathrm{y},\ \tfrac{i\omega}{M_\mathrm{s}}(\hat{\chi}\cdot\mathbf{h}_\mathrm{rf})_\mathrm{z}\right) \tag{S35}$$

The corresponding $L_\mathrm{j}$ is

$$L_\mathrm{j} = -C(\sigma_\mathrm{d} + i\epsilon\sigma_\mathrm{f})\chi_\mathrm{zy}\cdot f. \tag{S36}$$

with the proportionality constant $C$

$$C = \frac{hL_{12}}{4eM_\mathrm{s}}\eta(\delta_\mathrm{s}, w_\mathrm{cc}). \tag{S37}$$

It has to be normalized with

$$\tilde{L}_\mathrm{j} = \frac{L_\mathrm{j}}{\chi_\mathrm{yy}+\chi_\mathrm{zz}} = \frac{L_\mathrm{j}}{i\chi_\mathrm{zy}(\epsilon+1/\epsilon)}. \tag{S38}$$

This model is valid for equal CPW driving field components along $\hat{\mathbf{e}}_\mathrm{y}$- and $\hat{\mathbf{e}}_\mathrm{z}$-direction. However in a FM, it has been shown [17–19], that screening currents in the sample can particularly attenuate the z-component of the driving field $\mathbf{h}_\mathrm{rf,z}$. To account for this effect, we introduce a variable screening factor $\zeta \in [0,1]$ and rewrite Eq. (S38) as:

$$\tilde{L}_\mathrm{j} = \frac{L_\mathrm{j}}{\chi_\mathrm{yy}+\zeta\chi_\mathrm{zz}} = \frac{L_\mathrm{j}}{i\chi_\mathrm{yz}(\epsilon+\zeta/\epsilon)}. \tag{S39}$$

Thus, in this geometry $\tilde{L}_\mathrm{j}$ takes the form

$$\begin{aligned}\tilde{L}_\mathrm{j} &= C\frac{[-(\mu_0H_\mathrm{ext}+\mu_0M_\mathrm{s})\sigma_\mathrm{f} + i\sqrt{\mu_0H_\mathrm{ext}(\mu_0H_\mathrm{ext}+\mu_0M_\mathrm{s})}\sigma_\mathrm{d}]}{(\mu_0H_\mathrm{ext}(1+\zeta)+\mu_0M_\mathrm{s})}\cdot f \\ &= C\cdot f\cdot[-\epsilon_\mathrm{r}(f)\sigma_\mathrm{f} + i\epsilon_\mathrm{i}(f)\sigma_\mathrm{d}].\end{aligned} \tag{S40}$$

Using this result, the in-plane correction factors $\epsilon_\mathrm{r}(f)$ and $\epsilon_\mathrm{i}(f)$ in Eq. (**??**) take the form

$$\begin{aligned}\epsilon_\mathrm{r}(f) &= \frac{(\mu_0H_\mathrm{ext}+\mu_0M_\mathrm{s})}{\mu_0H_\mathrm{ext}(1+\zeta)+\mu_0M_\mathrm{s}} \\ \epsilon_\mathrm{i}(f) &= \frac{\sqrt{\mu_0H_\mathrm{ext}(\mu_0H_\mathrm{ext}+\mu_0M_\mathrm{s})}}{\mu_0H_\mathrm{ext}(1+\zeta)+\mu_0M_\mathrm{s}}.\end{aligned} \tag{S41}$$

Note that as we sweep $\mu_0H_\mathrm{ext}$ in a narrow range around $\mu_0H_\mathrm{res}$, we obtain the explicit frequency dependence of $\epsilon_\mathrm{r}(f)$ and $\epsilon_\mathrm{i}(f)$ by plugging Eq. (S15) $\mu_0H_\mathrm{ext} = \mu_0H_\mathrm{res}(f)$ into Eq. (S41). By applying this data procedure, we are hence able to extract the field- and damping-like current-induced torque conductivities $\sigma_\mathrm{f}$ and $\sigma_\mathrm{d}$ out of our bbFMR raw data from the obtained frequency-dependence of $\tilde{L}$. Apart from the different measurement geometry, the data analysis procedure outlined so far is equivalent to Berger et. al. in Ref. [16]. We only need to account in the in-plane measurement geometry for two susceptibility components ($\chi_\mathrm{zz}$ and $\chi_\mathrm{yy}$).

## 6. CHANGES TO THE DATA ANALYSIS PROCEDURE OF BERGER IN THE SUPERCONDUCTING STATE

We will now explain the changes to adapt the existing theory for the application of superconducting materials instead of normal metals.

- First and foremost we must account for the different strength of the oscillatory driving field $h_\mathrm{rf}$ below $T_\mathrm{c}$ due to superconducting image currents. We note that $h_\mathrm{rf}$ scales quadratically with the magnitude of the inductive coupling strength $\tilde{L}_0$ [see Eq.(S25)], while $\tilde{L}_\mathrm{j} \propto \partial\mathbf{m}/\partial t \propto h_\mathrm{rf}$ is linear in $h_\mathrm{rf}$. Thus, we must normalize our $\tilde{L}_\mathrm{SC}$ by multiplying the square root of the experimentally determined enhancement factor $\tilde{L}_0^\mathrm{SC}/\tilde{L}_0$. The resulting inductive coupling to SC $\tilde{L}_\mathrm{SC}$ takes the form

$$\begin{aligned}\mathrm{Re}(\tilde{L}_\mathrm{j}) &= -C\sqrt{\frac{\tilde{L}_0^\mathrm{SC}}{\tilde{L}_0}}\cdot\sigma_\mathrm{f}\epsilon_\mathrm{r}(f)\cdot f \\ \mathrm{Im}(\tilde{L}_\mathrm{j}) &= C\sqrt{\frac{\tilde{L}_0^\mathrm{SC}}{\tilde{L}_0}}\cdot\sigma_\mathrm{d}\epsilon_\mathrm{i}(f)\cdot f\end{aligned} \tag{S42}$$

. With this, our final fitting result for $\tilde{L}_{\mathrm{j}}$ is defined as:

$$\tilde{L}_{\mathrm{j}} = \begin{cases} C \cdot \sqrt{\tilde{L}_0^{\mathrm{SC}}/\tilde{L}_0} \cdot f \cdot [-\epsilon_{\mathrm{r}}(f)\sigma_{\mathrm{f}} + i\epsilon_{\mathrm{i}}(f)\sigma_{\mathrm{d}}] \ , & \text{for } \ T \leq T_{\mathrm{c}} \\ C \cdot f \cdot [-\epsilon_{\mathrm{r}}(f)\sigma_{\mathrm{f}} + i\epsilon_{\mathrm{i}}(f)\sigma_{\mathrm{d}}] \ , & \text{for } \ T > T_{\mathrm{c}}. \end{cases} \tag{S43}$$

- According to the results of Berger *et. al.* [16], the contribution of Faraday currents to $\sigma^{\mathrm{SOT}}$ is reciprocally proportional to the effective surface impedance $Z_{\mathrm{eff}}$, assumed to be constant with frequency. To include superconductors we insert the imaginary part of $Z_{\mathrm{eff}}$ from Eq. (S2) into the formula for $\sigma_{\mathrm{f}}^{\mathrm{F}}$ derived by Berger *et. al.*

$$\sigma_{\mathrm{f}}^{\mathrm{F}} = \frac{e\mu_0 M_{\mathrm{s}} d_{\mathrm{FM}}}{\hbar Z_{\mathrm{eff}}(f)} = i \cdot \frac{e M_{\mathrm{s}} d_{\mathrm{FM}} \cdot d_{\mathrm{SC}}}{h f \lambda_{\mathrm{L}}^2}. \tag{S44}$$

Here, we note that including the full expression from Eq. (S2) in our fitting procedure with realistic values for $\sigma_0$ and $\lambda_{\mathrm{L}}$ has a negligible impact on the extracted $\sigma_{\mathrm{SOT}}$ and was hence omitted to decrease the number of free parameters. The resulting $\sigma_{\mathrm{f}}^{\mathrm{F}}$ scales inversely with $f$ and thus when plugging it into Eq. (S42), its frequency dependence cancels out. The resulting contribution of Faraday currents to $\tilde{L}$ takes the form

$$\tilde{L}_{\mathrm{F}} = iC \frac{e M_{\mathrm{s}} d_{\mathrm{FM}} \cdot d_{\mathrm{SC}}}{h \lambda_{\mathrm{L}}^2(T)} \sqrt{\frac{\tilde{L}_0^{\mathrm{SC}}}{\tilde{L}_0}} \tag{S45}$$

Consequently, Faraday currents create an offset $\tilde{L}_{\mathrm{F}}$ in the imaginary part in the superconducting state. We do indeed observe a substantial y-axis intercept in Fig. S4. By plugging its magnitude into Eq. (S45), we obtain another method to extract the London penetration depth $\lambda_{\mathrm{L}}$. For the used samples it takes values ($1.5\mu\mathrm{m} \leq \lambda_{\mathrm{L}} \leq 3.5\mu\mathrm{m}$). These values are about a factor 2 larger than those extracted by fitting $|S_{21}|$. The performed fits with this adapted model match well with the extracted $\tilde{L}$ in real and imaginary part as indicated by the colored lines in Figs. S3 and S4. In the normal state (Fig. S3), the extracted $\tilde{L}$ can be well fitted with a quasi-linear inductive analysis model and the extracted $\sigma_{\mathrm{d}}$ have the right polarity and the expected magnitude in each of the samples. Furthermore, our modified model can explain the enhanced offset for our raw data in the imaginary part in the SC state (Fig. S4).

## 7. NORMALIZED INDUCTANCE AT ROOM TEMPERATURE

We start by illustrating the raw data of the normalized complex inductance $\tilde{L}$ for all four samples in the main text at $T = 300$ K in real and imaginary part in Fig. S3.

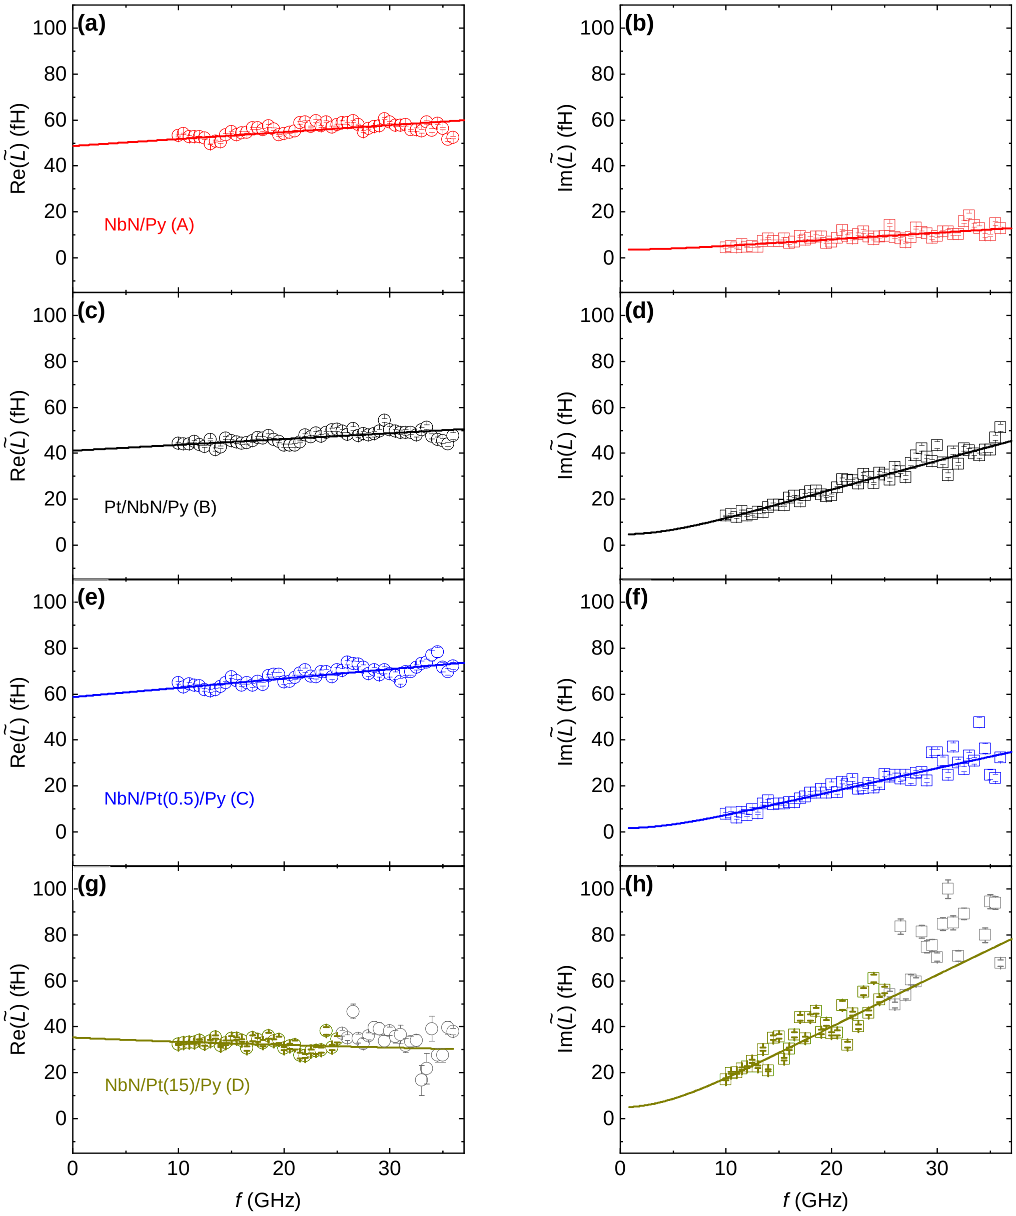


Figure S3. Real and imaginary part of the normalized inductance $\tilde{L}$ at room temperature for all the investigated samples. The ones comprising Pt exhibit a large iSHE as apparent from the slope of Im($\tilde{L}$) in (b),(f) and (h). Due to the enhanced damping in the NbN/thick Pt/Py-trilayer (sample D), the strongly broadened FMR-linewidths above 25 GHz lead to an imprecise amplitude extraction with large scattering. Hence these data-points have been omitted in the fitting of $\tilde{L}$. In Fig. S3, they are shown as gray data points. The y-axis intercept denoting the inductive coupling strength $L_0$ is similar in all samples. Lines in the graphs are fits to the data using Eq. (S28).

The real parts of the normalized inductive coupling strength Re($\tilde{L}$) in Fig. S3 have a similar y-axis intercept for all of the samples and exhibit a linear frequency dependence. For its imaginary part Im($\tilde{L}$), the samples display different behaviors. Sample B exhibits a large positive slope, while the sample without platinum shows only a minor positive slope. Both samples B and D have an intermediate positive slope. These results are in line with our expectations that

the slope in $\mathrm{Im}(\tilde{L})$ is governed by spin pumping into Pt and is hence the largest in samples containing thick Pt-layers and mostly absent in the red data points of sample A. All curves converge towards the origin for zero frequency, which is expected as in the dc limit [$f$ =0 Hz], the inductance must be strictly real. This condition is well met in our samples. However, we decided to refrain from rotating $\tilde{L} = (\mathrm{Re}(\tilde{L}), \mathrm{Im}(\tilde{L}))$ by a rotational matrix with angle $\beta$ to ensure $\mathrm{Im}(\tilde{L})(f = 0) = 0$ as performed in [16, 21]. Our reasoning is that the inductive coupling $\tilde{L}_0$ changes with temperature and we would hence generate artifacts in our temperature-dependent data, when rotating each data point with a slightly different angle $\beta$. Hence, we tolerate a minor $\mathrm{Im}(\tilde{L})$ offset in our fitting procedure.

## 8. NORMALIZED INDUCTANCE IN THE SUPERCONDUCTING STATE

We plot the normalized inductance of our samples (i.e. the y-axis intercept for $\mathrm{Re}(\tilde{L})$) at approx. $0.5 \times T_c$ in Fig. S4.

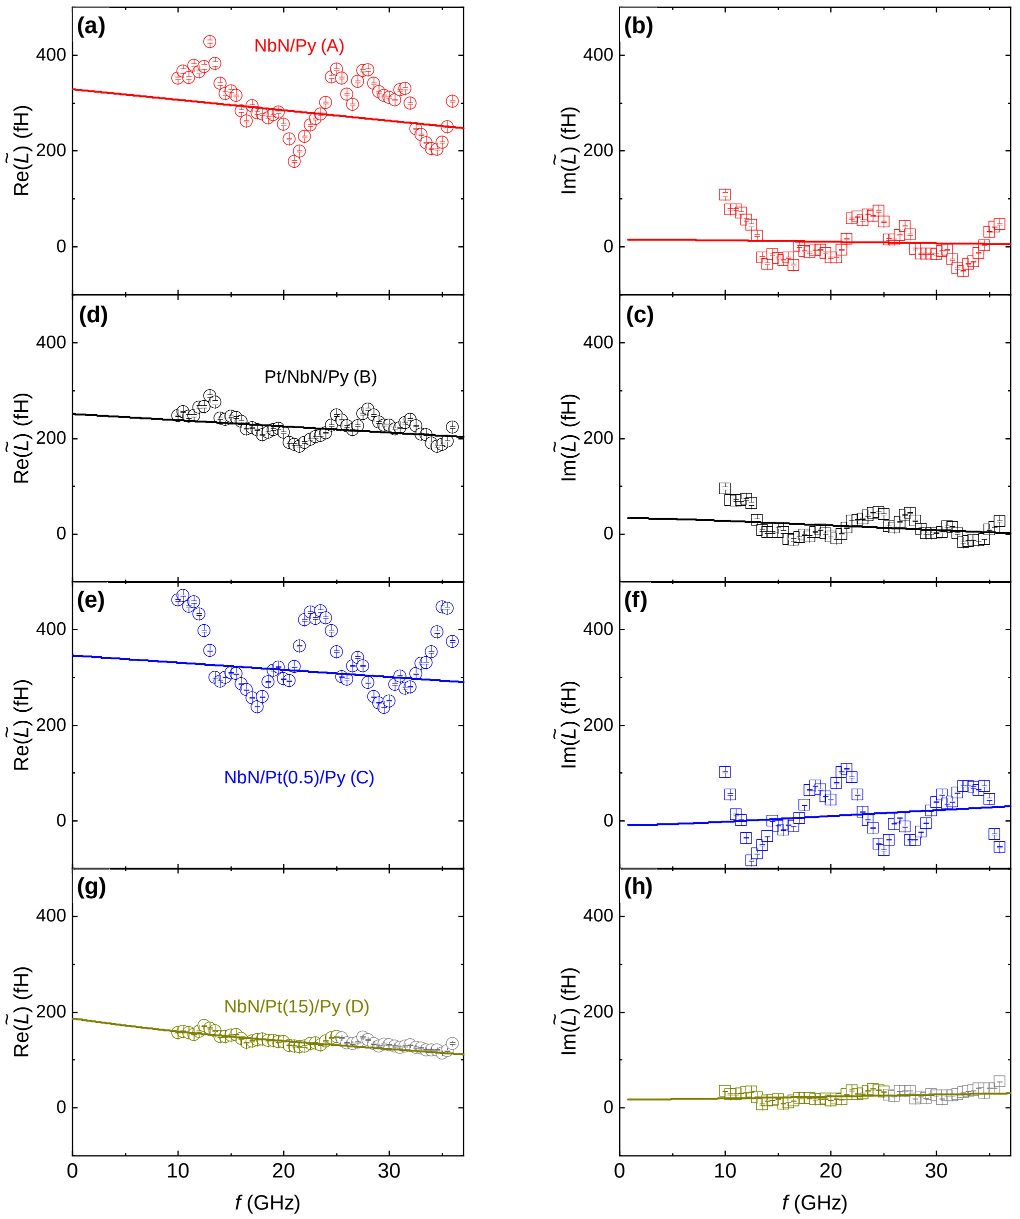


Figure S4. Real and imaginary part of the normalized inductance $\tilde{L}$ for the same samples below the superconducting transition temperature $T_c$. Dramatic changes in both $\tilde{L}_0$ and $L_j$ are apparent. The omitted data points for the NbN/thick Pt/Py-trilayer (sample D) are again shown as Grey data points, Lines in the graphs are fits to the data using Eq. (S28).

The observed enhancement of $\tilde{L}_0$ can be well explained by superconducting image charge currents repelling the oscillatory driving field of the CPW $\mathbf{h}_{\mathrm{rf}}$. Hence we are dealing with a system, where the ferromagnetic layer is exposed to driving fields from both the CC of a CPW at distance $\delta_s$, $h_{\mathrm{CPW}}$, and superconducting image currents flowing directly at its interface $h_{\mathrm{SC}}$. Moreover, we note that the CPW detects only the upper half of the flux $\mathbf{\Phi}_{\mathrm{dyn}}$ generated by the precessing macrospin $\mathbf{M}$ of the FM layer in the normal state. This fraction is enhanced below $T_C$, where the underlying superconductor expels the lower half of $\mathbf{\Phi}_{\mathrm{dyn}}$ from its interior via image currents and thereby essentially enhances the flux felt by the CPW. Consequently in the superconducting state the FM is not only driven with twice the driving field $\mathbf{h}_{\mathrm{rf}}$, enhancing the signal amplitude by a factor of 4, but the CPW also detects twice the net flux generated by the dynamically precessing $\mathbf{M}$. A 7-fold increase in FMR-amplitude has already been observed in samples containing thick Au backing layers instead of superconductors [4]. The observed slopes for $\tilde{L}$ in S4 are similar for all samples despite the varying stack sequences. We observe a reduction and sign change for Im($\tilde{\mathrm{L}}$), which indicates the blocking of spin currents and the iSHE in the SC state as well as slightly negative Re($\tilde{\mathrm{L}}$) corresponding

to a positive field-like current-induced torques $\sigma_{\mathrm{f}}$ of unknown origin. Moreover, an oscillatory behavior of $\tilde{L}$ in both real and imaginary part is apparent. The oscillatory features are reproducible and stable with temperature decaying only in magnitude $\tilde{L}_0$ for rising $T$. Superimposed on this pattern, a linear dependence on frequency can be extracted. Notably the results look similar for the samples with direct contact between SC and FM. In sample D, the inductive coupling $\mathrm{Re}(\tilde{L})$ is notably weaker as the increased distance between SC and FM reduces the enhancement effect of SC image currents. We note that this data set contains also less oscillatory features, which might indicate that the observed oscillatory variation with $f$ requires close SC/FM-proximity or direct contact. Here, we note the recent proposal of a perturbation-energy $\epsilon$-dependent Meißner response of SC material [22]. If we assume, this perturbation is the energy of the oscillatory rf-driving field $\epsilon = hf$ in our case, we can attribute the oscillatory features to a frequency-dependent Meißner response of the SC layer, where the non-vanishing time-dependent magnetic flux $\Phi$ is generated by the precessing magnetization of the FM layer on the one hand and dynamic charge currents generated via dynamic charge currents in adjacent SC/NM layers on the other hand.

## 9. MAGNETIZATION DYNAMICS PARAMETERS OF THE NBN/PY-THIN FILMS

In the main text, we illustrated the changes in Gilbert damping $\alpha$ of our samples in the superconducting state. Here we also show the full temperature range from $T \ll T_{\mathrm{c}}$ to RT of the raw magnetization dynamics parameters ($g$-factor, $M_{\mathrm{eff}}$, $\alpha$ and $H_{\mathrm{inh}}$), extracted by fitting the raw data $\Delta S_{21}(f)$ to Eqs. (S15) and (S17), in Fig. S5. As evident from Fig. S5(a), the $g$-factor is identical for all samples and exhibits no strong temperature dependence. The effective magnetization $\mu_0 M_{\mathrm{eff}}$ in Fig. S5(b) increases with decreasing $T$, which we attribute to the increase in saturation magnetization with decreasing temperature. The Gilbert damping $\alpha$ in Fig. S5(c) is higher in samples, where Py is directly grown on Pt due to increased spin pumping and sizable spin memory loss in these samples [21, 23]. The observed temperature dependence of $\alpha$ in the normal state matches previous results [24] and theoretical predictions [25]. The reduction of $\alpha$ below $T_{\mathrm{c}}$ is due to altered spin transport properties of SC. For $\mu_0 H_{\mathrm{inh}}$ in Fig. S5(d) we detect the manifestation of a sizable $\mu_0 H_{\mathrm{inh}}$ for temperatures slightly above $T_{\mathrm{c}}$ for all samples. The further changes in $\mu_0 H_{\mathrm{inh}}$ below $T_{\mathrm{c}}$ are likely caused by an incoherent precession of $\mathbf{M}$ at the FM/SC-interface as proposed in [26]. Overall the spectroscopic parameters of Py exhibit only minor changes with $T$ in the normal states.

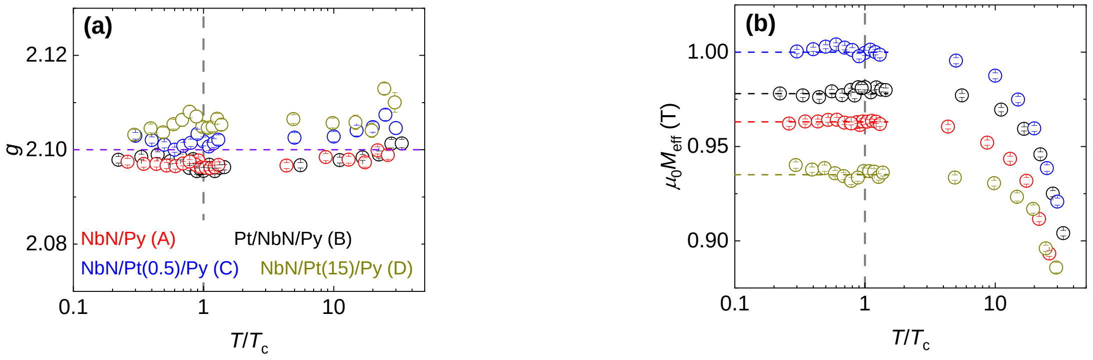

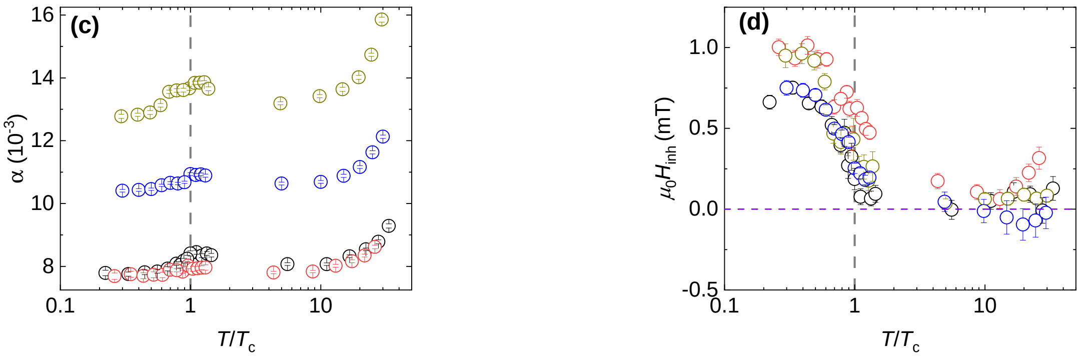


Figure S5. Temperature dependence of spectroscopic parameters for the NbN/Py-samples. (a): The $g$-factor displays no clear dependence on T, while the effective magnetization $\mu_0 M_{\mathrm{eff}}$ decreases for increasing temperature due to the thermal excitation of magnons. (c) and (d) illustrate the changes of the Gilbert damping $\alpha$ and inhomogeneous broadening $\mu_0 H_{\mathrm{inh}}$, respectively.

## 10. INVERSE CURRENT-INDUCED TORQUES AS FUNCTION OF TEMPERATURE

In Fig. S6 we plot the entire recorded temperature range for field- and damping-like $\sigma^{\mathrm{SOT}}$ on a logarithmic scale.

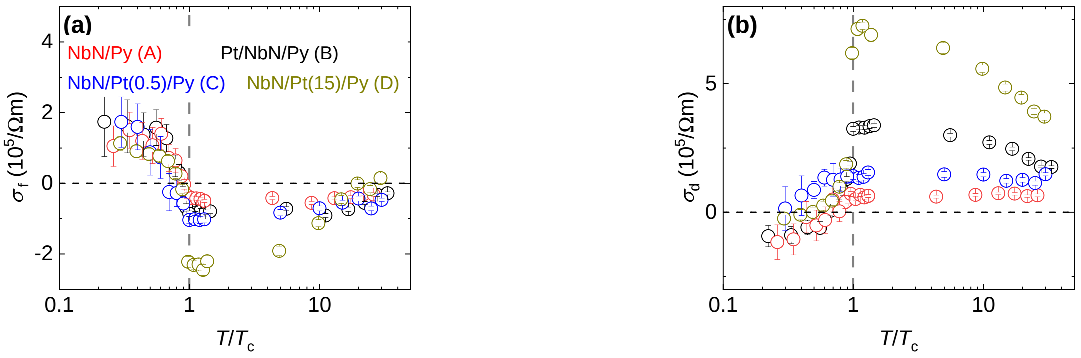


Figure S6. Extracted field (a) and damping-like (b) current-induced torques $\sigma_{\mathrm{f}}$ and $\sigma_{\mathrm{d}}$ plotted as a function of $T$ extracted for a broad range of temperatures spanning from RT to $T \ll T_{\mathrm{C}}$. The extracted $\sigma^{\mathrm{SOT}}$ are extracted by fitting our raw data to S43.

Both iSOT parameters remain roughly constant in the normal state for all samples except for the NbN/thick Pt/Py- and Pt/NbN/Py-trilayers (samples B and D). Here, we observe a decrease in the magnitude of both $\sigma_{\mathrm{d}}$ and $\sigma_{\mathrm{f}}$ with increasing temperature. We attribute the former to enhanced spin pumping (higher $\sigma_{\mathrm{d}}$) and the latter to stronger Faraday currents in Pt for low temperatures, both originating from the increase in conductivity of Pt with decreasing temperature. As discussed in the main text, we observe large changes in the $\sigma^{\mathrm{SOT}}$ in the superconducting state. Starting our discussion with the field-like $\sigma_{\mathrm{f}}$ in Fig. S6(a), we note that all samples exhibit equal $\sigma_{\mathrm{f}}$ at room temperature. We attribute their growing divergence with reducing $T$ to a stronger contribution of Faraday currents in the Pt layer due to an increase in Pt conductivity with decreasing temperature. In sample D, we observe the strongest changes in $\sigma_{\mathrm{f}}$ with temperature $T > T_{\mathrm{c}}$, which are absent in the samples including only thin or no Pt. By investigating the magnitude for sample A, the impact of $\sigma_{\mathrm{f}}$ can be assumed to be very low in the normal state. The magnitude of the damping-like $\sigma_{\mathrm{d}}$ rises with the thickness of the Pt layer in our samples. We attribute the low positive $\sigma_{\mathrm{d}}$ in the red data points of sample A to minor spin pumping into the unoxidized fraction of the Ta-caplayer. Here the negative spin Hall angle in Ta combined with the opposite spin current injection direction give rise to a net positive $\sigma_{\mathrm{d}}$. We also observe more efficient spin pumping into Pt at lower temperatures, which can also be explained by its enhanced conductivity at cryogenic temperatures.

## 11. DETECTED QMISHE IN SC/FM-HETEROSTRUCTURES IN COMPARISON TO [27]

As briefly discussed in the main text, one possible scenario for the finite negative $\sigma_\mathrm{d}$ in our experiments for $T < T_\mathrm{c}$ is the Quasiparticle mediated inverse spin Hall effect (QMiSHE) [28–31]. First experiments conducted by Wakamura et al. utilizing non-local lateral spin injection techniques, showed greatly enhanced iSHE voltage for T approaching zero. In our case we find a saturation of $\sigma_\mathrm{d}$ for very low temperatures. This discrepancy may be explained by the difference in detection techniques: We are able to detect the flux generated by the dynamic $\mathbf{J}_\mathrm{q}$ (caused by the spin-to-charge current conversion of the QMiSHE) as a change in inductive coupling strength between sample and CPW, whereas Wakamura *et. al.* [27] measured the accumulation of electron- and hole-like quasiparticle (QP) on opposite sides of his superconducting NbN strips as a voltage signal.

For nonlocal devices the spin Hall resistance $\Delta R_\mathrm{SH}$ generated by quasiparticles is proportional to both quasiparticle resistance $\rho_\mathrm{qp}$ and spin Hall angle $\Theta_\mathrm{SH}$. Following [27, 32], the former can be obtained by normalizing the normal state longitudinal resistance $\rho_\mathrm{long}$ to the amount of QP populated above the superconducting gap $\Delta$. This contribution is governed by the Fermi distribution $f_0(\Delta(T))$

$$\rho_\mathrm{qp} = \rho_\mathrm{long}/[2f_0(\Delta(T))]. \tag{S46}$$

From this expression the increase in $\rho_\mathrm{qp}$ for low temperatures immediately becomes apparent, as the Fermi distribution takes lower values for rising gap values $\Delta(T)$. The spin Hall angle $\Theta_\mathrm{SH}$ comprises extrinsic contributions from side jump (SJ)- and skew scattering (SS) as well as intrinsic effects [33]. Taking these three contributions into account, the Hall resistivity $\rho_\mathrm{SH}$ scales with the longitudinal resistivity $\rho_\mathrm{long}$ according to:

$$\rho_\mathrm{SH} = a\rho_\mathrm{long} + b\rho_\mathrm{long}^2, \tag{S47}$$

where $a$ and $b$ are proportionality constants quantifying the impact of skew scattering ($a$) and SJ-scattering plus intrinsic effects ($b$), respectively [27].

The spin Hall angle is defined as the ratio between Spin-Hall and longitudinal resistance $\Theta_\mathrm{SH} = \rho_\mathrm{SH}/\rho_\mathrm{long}$ and hence takes the form

$$\Theta_\mathrm{SH} = a + b\rho_\mathrm{long}. \tag{S48}$$

In the SC state, we replace $\rho_\mathrm{long}$ with the QP resistance $\rho_\mathrm{qp}$. Hence, the intrinsic and side-jump contributions to $\Theta_\mathrm{SH}$ diverge with $\rho_\mathrm{qp}$ for decreasing $T$ in the SC state.

As a result, in non-local spin current experiments, a dramatically enhanced spin Hall resistance $\Delta R_\mathrm{SH} \propto \rho_\mathrm{qp}\Theta_\mathrm{SH}$ as observed by Wakamura *et. al.* is in agreement with theoretical predictions.

In contrast, in our experiments we measure the flux generated by $\mathbf{j}_\mathrm{q}$ instead of $\Delta R_\mathrm{SH}$ (the open circuit voltage). For QP charge currents, the contributions of $\rho_\mathrm{qp}$ and $\Theta_\mathrm{SH}$ counteract each other. The corresponding damping-like $\sigma_\mathrm{d}$ is $\sigma_\mathrm{d} \propto \Theta_\mathrm{SH}/\rho_\mathrm{qp}$ in accordance to [16]. Consequently, its net temperature dependence cancels out, leading to a constant value for $\sigma_\mathrm{d}$. This theoretical prediction is in agreement with our results for $\sigma_\mathrm{d}$ in Fig. 3(b) of the main text, which appear to saturate at minor negative values for $T \to 0$. We attribute the negative sign to the negative spin Hall angle [34] and the associated QMiSHE in NbN.

In summary, by using existing theoretical models for the quasiparticle-mediated inverse spin Hall effect [QMiSHE], we can satisfactorily explain our results for the damping-like $\sigma_\mathrm{d}$ below $T_\mathrm{c}$. Deviations in the detected quantitative magnitude of this effect from results of Wakamura *et. al.* originate from the different applied detection methods.

## 12. CURRENT-INDUCED TORQUES IN SC-FM-HETEROSTRUCTURES USING ANOTHER FM

Apart from Permalloy, we additionally used the ultralow-damping FM $Co_{25}Fe_{75}$[35]. This material is very growth-sensitive and we were not able to grow $Co_{25}Fe_{75}$ on Pt while maintaining comparable magnetization dynamics parameters. We hence decided to vary the used bottom spin sink layer. We grew samples with stack sequence NM (5 nm)/NbN (16 nm)/$Co_{25}Fe_{75}$ (3 nm). The resulting magnetization dynamics parameters in the temperature range around $T_c$ are shown in Fig. S7.

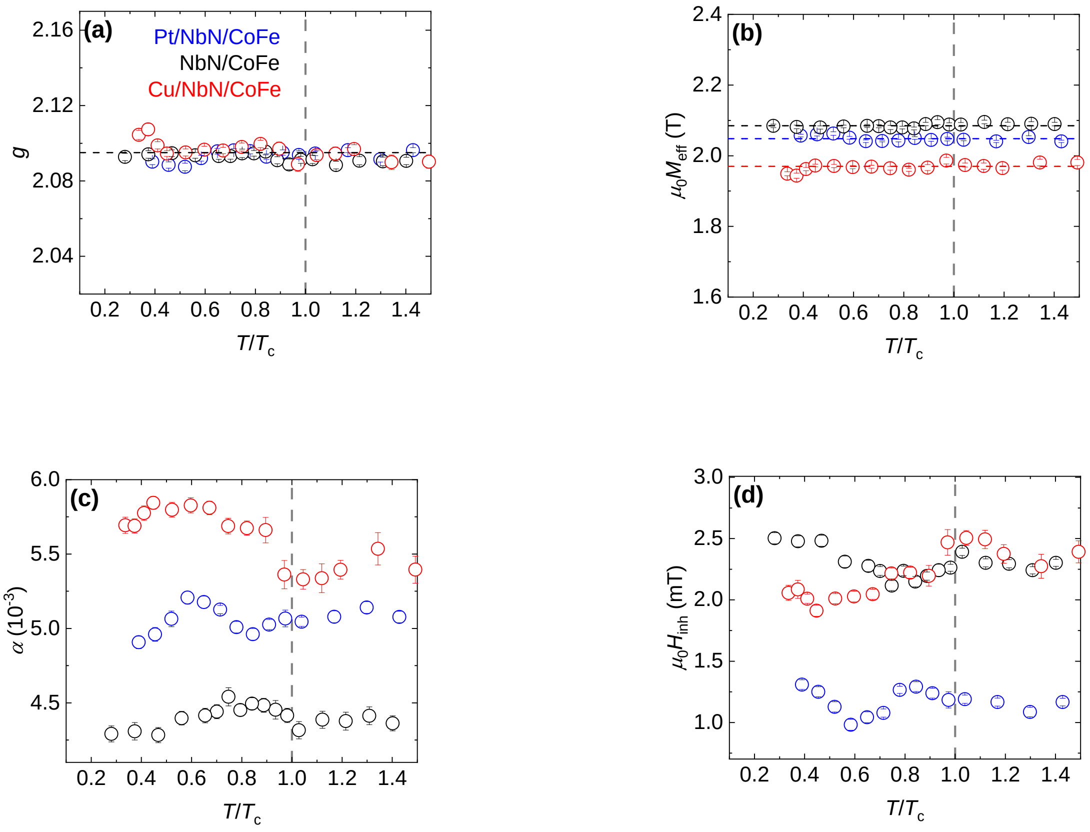


Figure S7. Magnetization dynamics parameters of NM/NbN/$Co_{25}Fe_{75}$-samples recorded in the temperature range of the superconducting $T_c$. Both the $g$-factor in (a) and effective magnetization in (b) exhibit no clear temperature dependence. For the Gilbert damping $\alpha$ in (c), we detect a minor coherence peak in all of the investigated samples. Moreover the inhomogeneous line-broadening in (d) is also altered below $T_c$.

Just like for the results for NbN/Py-samples, we observe no distinct temperature dependence in the effective $g$-factor in Fig. S7(a) nor in the effective magnetization $M_{\mathrm{eff}}$ in Fig. S7(b). However in Fig. S7(c), we do detect a minor coherence peak in Gilbert damping $\alpha$ [36, 37] for all samples contrary to the observed monotonic reduction of $\alpha$ in Py in the SC state. This indicates, that in SC/FM-heterostructures with different FM, entailing varying properties and spin diffusion lengths, one will observe different results for $\alpha$. Following the derivations in [36], the coherence peak magnitude is enhanced in SC/FM-interfaces with low mean free path $l$, spin diffusion length $\lambda_s$ and superconducting coherence length $\xi_0$. Consequently, we propose that 'dirty' SC/FM-interfaces give rise to a sizable coherence peak, while in clean interfaces, the characteristic reduction of $\alpha$ with reduced $T$ due to QP freeze-out is detected. The latter has for example been observed in Fig. 3(b) of the main text and in [38]. However, we note that the apparent correlation between $\alpha$ in Fig. S7(c) and $\mu_0 H_{\mathrm{inh}}$ in Fig. S7(d) hints at the potential impact of two-magnon scattering in our samples. All of our $\Delta H(f)$ data could be fitted linearly without any apparent deviations. However, we can not rule out the presence of a small but finite impact of two-magnon scattering on the linewidth $\Delta H(f)$.
Finally, we plot the extracted $\sigma^{\mathrm{SOT}}$ of our NbN/$Co_{25}Fe_{75}$-samples in Fig. S8 and compare them to the results in our main text.

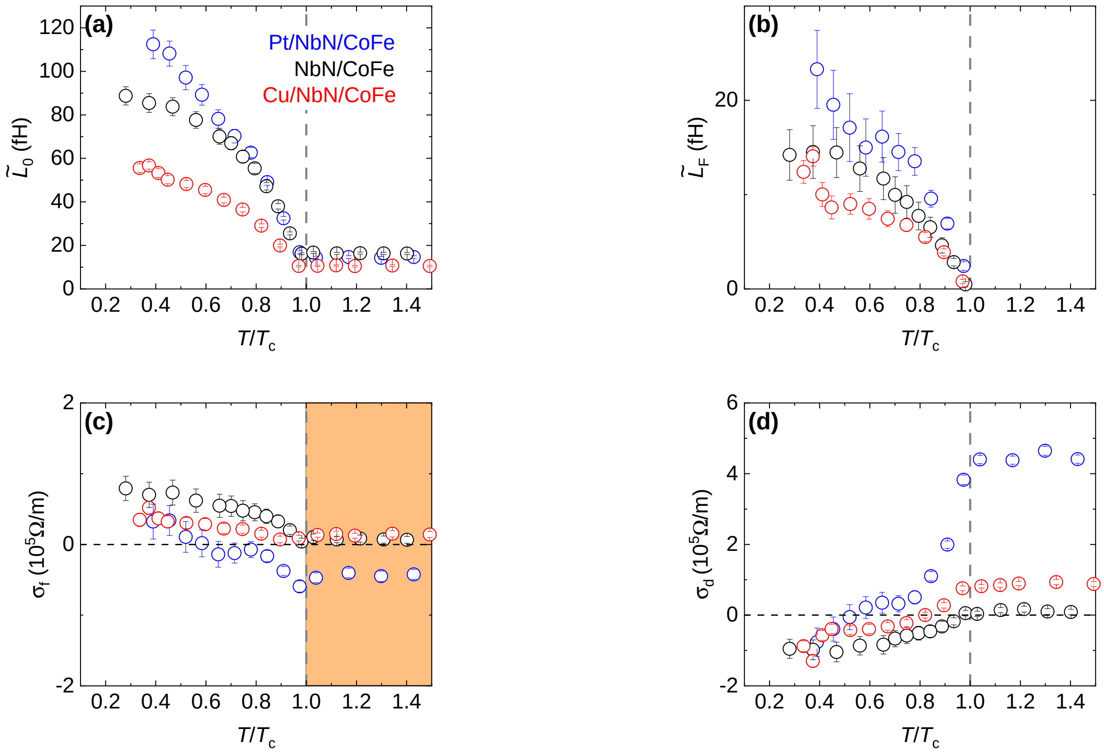


Figure S8. Inductive analysis results of NbN/$Co_{25}Fe_{75}$-samples recorded in the temperature range of $T_c$. In agreement with the obtained results for NbN/Py-heterostructures, we observe a dramatically enhanced $\mathrm{Re}(\tilde{L}_0)$ (a) below $T_c$. Superconducting Faraday-currents again give rise to an offset in $\tilde{L}_F$ in panel (b). In panel (c), we detect a sizable $\sigma_f$ in the superconducting state. (d): For the damping-like $\sigma_d$ above $T_c$ we extract a large positive value for the Pt/NbN/$Co_{25}Fe_{75}$-trilayer. In the superconducting state, we observe a saturation towards small negative values for all samples.

In similar fashion as for the results obtained NbN/Py-heterostructures, we observe a dramatically enhanced $\mathrm{Re}(\tilde{L}_0)$ in Fig. S8(a) below $T_c$. Additionally, the superconducting Faraday-currents give rise to an offset in $\mathrm{Im}(\tilde{L}_0)$ in Fig. S8(b), which is of comparable magnitude to that for NbN/Py-samples. In Fig. S8(c), we observe almost negligible $\sigma_f$ in the normal state. Below $T_c$, $\sigma_f$ increases with decreasing temperature towards positive value in agreement with our findings for the NbN/Py-samples. Moreover, we find a good quantitative agreement between the two sample series with different FMs. For the damping-like $\sigma_d$ in Fig. S8(d), we observe substantial positive values in the normal state for the Pt/NbN/$Co_{25}Fe_{75}$-trilayer. In the superconducting state, the $\sigma_d$ decreases to negative values with decreasing temperature. These results are in good agreement to those of our NbN/Py-samples and suggest quasiparticle mediated spin pumping even at low temperatures $T \ll T_c$ due to very large spin Hall angles [28] and a finite fraction of QP surviving even at $T = 0$ K [36].

## 13. CHOICE AND IMPACT OF OF $\zeta$ FOR OUR DATA ANALYSIS

In our experiments, we fit with $\zeta = 0$, as the FMR-signal for $H_{ext}$ along $\hat{\mathbf{e_y}}$ is greatly reduced in the normal state as illustrated in Fig. S9(a) and (b) in the real and imaginary part of $\Delta S_{21}$ respectively for sample B confirming that we can neglect the oop driving field in good approximation in our measurements.

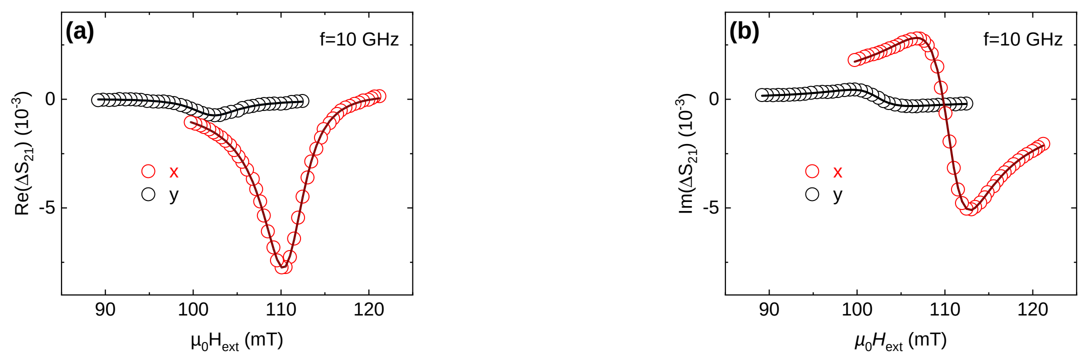


Figure S9. Background-corrected change of complex scattering parameter $\Delta S_{21}$ in resonance in both in-plane geometries (x: $\mathbf{H}_{ext}$ along CPW/ y: $\mathbf{H}_{ext}$ perpendicular to CPW) at $f$ =10 GHz at RT for sample B. The FMR is enhanced by a factor way larger than 2, which proofs that the oop-driving field component of the Polder-susceptibility $\chi_{zz}$ can be neglected. Deviation in resonance field position are due to trapped flux in the SC coils and imperfect geometric alignment in the y-direction.

We also note that the observed enhancement of inductive coupling in the SC-state due to the screening currents in the SC exclusively enhances the y-component of $\mathbf{h}_{rf}$ and simultaneously screens its z-component even more strongly. Likewise to the results at RT, the real and imaginary part of $\Delta S_{21}$ are shown in Fig. S10(a) and (b). Thus, $\zeta = 0$ is a good approximation below $T_c$.

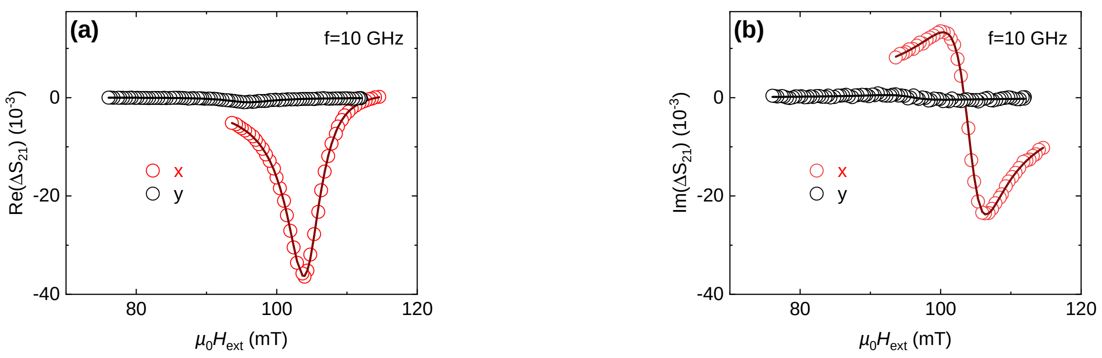


Figure S10. Background-corrected change of complex scattering parameter $\Delta S_{21}$ in resonance in both in-plane geometries (x: $\mathbf{H}_{ext}$ along CPW/ y: $\mathbf{H}_{ext}$ perpendicular to CPW ) at $f$ =10 GHz at $T = 5$ K for sample B. The FMR is enhanced in x- and attenuated in the y-direction in the SC state. Consequently, the relative disparity between their respective magnitudes is even larger than at RT.

From these results, we deduce, that our assumption of $\zeta = 0$ is valid in our experiments. To obtain a relative estimate of the changes in $\sigma_{SOT}$ induced by varying $\zeta$, we plot the full temperature range for field- and damping-like current-induced torques of sample B in Fig. S11(a) and (b) for the extreme cases $\zeta = 1$ (red) and $\zeta = 0$ (blue).

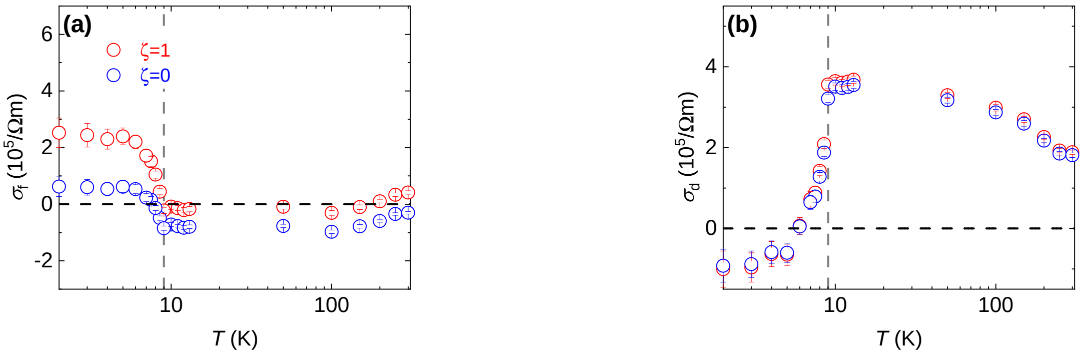


Figure S11. Field-like (a) and damping-like (b) $\sigma^{\mathrm{SOT}}$ for both limiting cases $\zeta = 1$ and $\zeta = 0$ for the Pt/NbN/Py-trilayer sample (sample B) plotted over the full temperature range on a logarithmic scale.

From Fig. S11(a), we can deduce, that while changing the parameter $\zeta$ leads to quantitative changes in the field-like current-induced torques, its overall evolution with temperature and in particular its dramatic change in the SC state are independent of $\zeta$. The damping-like$\sigma_{\mathrm{d}}$ in Fig. S11(b) remains almost unchanged. These results proof, that the results for our $\sigma^{\mathrm{SOT}}$ are not artifacts of a faulty fitting procedure, but indeed preserved for varying values of $\zeta$.

* manuel.mueller@wmi.badw.de
† matthias.althammer@wmi.badw.de

[1] G. Horn and E. Saur, Präparation und Supraleitungseigenschaften von Niobnitrid sowie Niobnitrid mit Titan-, Zirkon- und Tantalzusatz, Zeitschrift für Phys. A Hadron. Nucl. **210**, 70 (1968).
[2] D. Hazra, N. Tsavdaris, S. Jebari, A. Grimm, F. Blanchet, F. Mercier, E. Blanquet, C. Chapelier, and M. Hofheinz, Superconducting properties of very high quality NbN thin films grown by high temperature chemical vapor deposition, Supercond. Sci. Technol. **29**, 105011 (2016).
[3] M. Chand, A. Mishra, Y. M. Xiong, A. Kamlapure, S. P. Chockalingam, J. Jesudasan, V. Bagwe, M. Mondal, P. W. Adams, V. Tripathi, and P. Raychaudhuri, Temperature dependence of resistivity and Hall coefficient in strongly disordered NbN thin films, Phys. Rev. B **80**, 134514 (2009).
[4] H. Głowiński, M. Schmidt, I. Gościańska, J.-P. Ansermet, and J. Dubowik, Coplanar waveguide based ferromagnetic resonance in ultrathin film magnetic nanostructures: Impact of conducting layers, J. Appl. Phys. **116**, 053901 (2014).
[5] G. Ciovati, AC/RF superconductivity, CAS-CERN Accelerator School: Superconductivity for Accelerators - Proceedings **005**, 57 (2014).
[6] Y. Imai, H. Takahashi, K. Kitagawa, K. Matsubayashi, N. Nakai, Y. Nagai, Y. Uwatoko, M. Machida, and A. Maeda, Microwave Surface Impedance Measurements of LiFeAs Single Crystals, Journal of the Physical Society of Japan **80**, 013704 (2011).
[7] A. I. Gubin, K. S. Il'in, S. A. Vitusevich, M. Siegel, and N. Klein, Dependence of magnetic penetration depth on the thickness of superconducting Nb thin films, Phys. Rev. B **72**, 064503 (2005).
[8] C. Gorter and H. Casimir, On supraconductivity I, Physica **1**, 306 (1934).
[9] B. Mühlschlegel, Die thermodynamischen Funktionen des Supraleiters, Zeitschrift für Phys. **155**, 313 (1959).
[10] S. P. Chockalingam, M. Chand, J. Jesudasan, V. Tripathi, and P. Raychaudhuri, Superconducting properties and Hall effect of epitaxial NbN thin films, Phys. Rev. B **77**, 214503 (2008).
[11] Y. Yao, Q. Song, Y. Takamura, J. P. Cascales, W. Yuan, Y. Ma, Y. Yun, X. C. Xie, J. S. Moodera, and W. Han, Probe of spin dynamics in superconducting NbN thin films via spin pumping, Phys. Rev. B **97**, 224414 (2018).
[12] E. Silva, N. Pompeo, and O. V. Dobrovolskiy, Vortices at Microwave Frequencies, Phys. Sci. Rev. **2**, 1 (2017).
[13] T. Gilbert, Classics in Magnetics A Phenomenological Theory of Damping in Ferromagnetic Materials, IEEE Trans. Magn. **40**, 3443 (2004).
[14] D. Polder, On the theory of ferromagnetic resonance, Physica **15**, 253 (1949).
[15] H. T. Nembach, T. J. Silva, J. M. Shaw, M. L. Schneider, M. J. Carey, S. Maat, and J. R. Childress, Perpendicular ferromagnetic resonance measurements of damping and Landé g-factor in sputtered $(Co_2Mn)_{1-x}Ge_x$ thin films, Phys. Rev. B , 054424.
[16] A. J. Berger, E. R. Edwards, H. T. Nembach, A. D. Karenowska, M. Weiler, and T. J. Silva, Inductive detection of fieldlike and dampinglike ac inverse spin-orbit torques in ferromagnet/normal-metal bilayers, Phys. Rev. B **97**, 94407 (2018).
[17] I. S. Maksymov and M. Kostylev, Impact of conducting nonmagnetic layers on the magnetization dynamics in thin-film magnetic nanostructures, Journal of Applied Physics **113**, 043927 (2013).
[18] I. S. Maksymov and M. Kostylev, Microwave eddy-current shielding effect in metallic films and periodic nanostructures of sub-skin-depth thicknesses and its impact on stripline ferromagnetic resonance spectroscopy, Journal of Applied Physics **116** (2014).
[19] M. Kostylev, Strong asymmetry of microwave absorption by bilayer conducting ferromagnetic films in the microstrip-line based broadband ferromagnetic resonance, Journal of Applied Physics **106**, 043903 (2009).
[20] E. B. Rosa, The self and mutual-inductances of linear conductors, Bull. Bur. Stand. **4**, 301 (1908).
[21] A. J. Berger, E. R. J. Edwards, H. T. Nembach, O. Karis, M. Weiler, and T. J. Silva, Determination of the spin Hall effect and the spin diffusion length of Pt from self-consistent fitting of damping enhancement and inverse spin-orbit torque measurements, Phys. Rev. B **98**, 024402 (2018).
[22] J. A. Ouassou, W. Belzig, and J. Linder, Prediction of a Paramagnetic Meissner Effect in Voltage-Biased Superconductor–Normal-Metal Bilayers, Physical Review Letters **124**, 047001 (2020).
[23] J.-C. Rojas-Sánchez, N. Reyren, P. Laczkowski, W. Savero, J.-P. Attané, C. Deranlot, M. Jamet, J.-M. George, L. Vila, and H. Jaffrès, Spin Pumping and Inverse Spin Hall Effect in Platinum: The Essential Role of Spin-Memory Loss at Metallic Interfaces, Phys. Rev. Lett. **112**, 106602 (2014).
[24] L. Frangou, G. Forestier, S. Auffret, S. Gambarelli, and V. Baltz, Relaxation mechanism in NiFe thin films driven by spin angular momentum absorption throughout the antiferromagnetic phase transition in native surface oxides, Physical Review B **95**, 054416 (2017).
[25] K. Gilmore, Y. U. Idzerda, and M. D. Stiles, Identification of the dominant precession-damping mechanism in Fe, Co, and Ni by first-principles calculations, Physical Review Letters **99**, 1 (2007).
[26] K.-r. Jeon, C. Ciccarelli, H. Kurebayashi, L. F. Cohen, X. Montiel, M. Eschrig, T. Wagner, S. Komori, A. Srivastava, J. W. Robinson, and M. G. Blamire, Effect of Meissner Screening and Trapped Magnetic Flux on Magnetization Dynamics in Thick $Nb/Ni_{80}Fe_{20}/Nb$ Trilayers, Phys. Rev. Appl. **11**, 014061 (2019).
[27] T. Wakamura, H. Akaike, Y. Omori, Y. Niimi, S. Takahashi, A. Fujimaki, S. Maekawa, and Y. Otani, Quasiparticle-mediated spin Hall effect in a superconductor, Nat. Mater. **14**, 675 (2015).
[28] S. Takahashi and S. Maekawa, Spin Hall Effect in Superconductors, Jpn. J. Appl. Phys. **51**, 010110 (2012).

[29] S. Takahashi and S. Maekawa, Spin Current in Metals and Superconductors, J. Phys. Soc. Japan **77**, 031009 (2008).
[30] H. Kontani, J. Goryo, and D. S. Hirashima, Intrinsic Spin Hall Effect in the <math display="inline"> <mi>s</mi> </math> -Wave Superconducting State: Analysis of the Rashba Model, Phys. Rev. Lett. **102**, 086602 (2009).
[31] S. Takahashi and S. Maekawa, Hall Effect Induced by a Spin-Polarized Current in Superconductors, Phys. Rev. Lett. **88**, 116601 (2002).
[32] S. Takahashi, T. Yamashita, H. Imamura, and S. Maekawa, Spin-relaxation and magnetoresistance in FM/SC/FM tunnel junctions, J. Magn. Magn. Mater. **240**, 100 (2002).
[33] S. Onoda, N. Sugimoto, and N. Nagaosa, Intrinsic Versus Extrinsic Anomalous Hall Effect in Ferromagnets, Physical Review Letters **97**, 126602 (2006).
[34] K. Rogdakis, A. Sud, M. Amado, C. M. Lee, L. McKenzie-Sell, K. R. Jeon, M. Cubukcu, M. G. Blamire, J. W. A. Robinson, L. F. Cohen, and H. Kurebayashi, Spin transport parameters of NbN thin films characterized by spin pumping experiments, Phys. Rev. Mater. **3**, 014406 (2019).
[35] L. Flacke, L. Liensberger, M. Althammer, H. Huebl, S. Geprägs, K. Schultheiss, A. Buzdakov, T. Hula, H. Schultheiss, E. R. J. Edwards, H. T. Nembach, J. M. Shaw, R. Gross, and M. Weiler, High spin-wave propagation length consistent with low damping in a metallic ferromagnet, Applied Physics Letters **115**, 122402 (2019).
[36] M. Inoue, M. Ichioka, and H. Adachi, Spin pumping into superconductors: A new probe of spin dynamics in a superconducting thin film, Phys. Rev. B **96**, 024414 (2017).
[37] T. Kato, Y. Ohnuma, M. Matsuo, J. Rech, T. Jonckheere, and T. Martin, Microscopic theory of spin transport at the interface between a superconductor and a ferromagnetic insulator, Phys. Rev. B **99**, 144411 (2019).
[38] C. Bell, S. Milikisyants, M. Huber, and J. Aarts, Spin Dynamics in a Superconductor-Ferromagnet Proximity System, Phys. Rev. Lett. **100**, 047002 (2008).
